# Supplementary material for: Ultrafast Multi-Shot Ablation and Defect Generation in Monolayer Transition Metal Dichalcogenides
Source: arXiv:2112.10743 source file (2021-12-20)
Supplement: Supplementary file 1 [file SI.pdf]

**Supporting Information:**

# Ultrafast Multi-Shot Ablation and Defect Generation in Monolayer Transition Metal Dichalcogenides

Joel M. Solomon,[1] Sabeeh Irfan Ahmad,[1] Arpit Dave,[1] Li-Syuan Lu,[2,3] Yu-Chen Wu,[2] Wen-Hao Chang,[2,3] Chih-Wei Luo,[2,4,5] and Tsing-Hua Her[1]

1) *Department of Physics and Optical Science, The University of North Carolina at Charlotte, Charlotte, North Carolina, 28223, United States*

2) *Department of Electrophysics, National Yang Ming Chiao Tung University, Hsinchu 30010, Taiwan*

3) *Research Center for Applied Sciences, Academia Sinica, Taipei 11529, Taiwan*

4) *Institute of Physics and Center for Emergent Functional Matter Science, National Yang Ming Chiao Tung University, Hsinchu 30010, Taiwan*

5) *National Synchrotron Radiation Research Center (NSRRC), Hsinchu 30076, Taiwan*

(*Electronic mail: ther@uncc.edu)

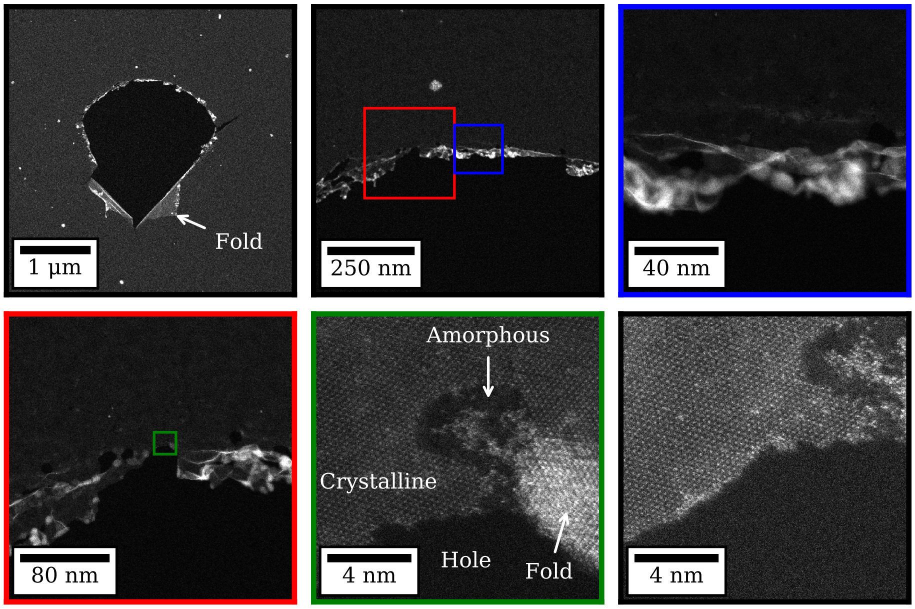


FIG. S1: HR-TEM images of a hole created in a suspended monolayer $MoS_2$ film by a single ultrafast pulse with $F = 2.0F_{th}(1)$.

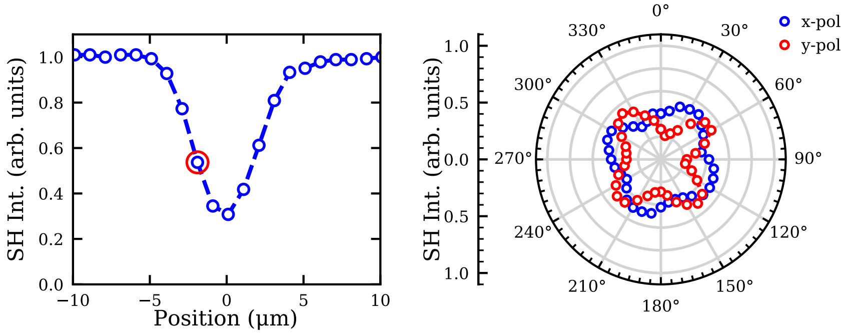


FIG. S2: (left) SH line scan across a hole in an $MoS_2$ film caused by a single pulse with $F = 2.0F_{th}(1)$. The SH intensity does not go to zero since the probe pulse spot size is larger than the hole size. (right) The SH polar profile recorded at the spot marked with the red circle in the line scan.

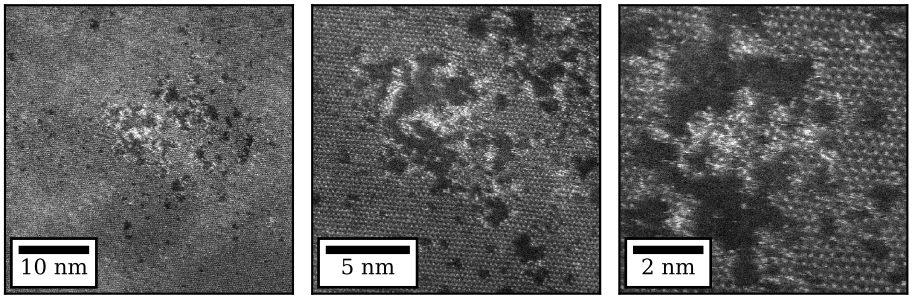


FIG. S3: HR-TEM images of a suspended monolayer $MoS_2$ film excited by a single pulse with $F = F_{th}(1)$.
